# Supplementary material for: InfTDA: A Simple TopDown Mechanism for Hierarchical Differentially Private Counting Queries
Source: arXiv:2505.05347 source file (2025-05-08)
Supplement: Supplementary file 1 [file Usefull_inequalities.tex]

\section{Usefull Inequalities}
\begin{corollary}[Corollary 9 \cite{canonne2020discrete}]
\label{corollary: discrete Gaussian tail}
Let $Z\sim \mathcal{N}_{\mathbb{Z}}(0, \sigma^2)$. Then $\textnormal{Var}[Z]\leq \sigma^2$ and $\textnormal{Pr}[Z\geq t]\leq e^{-\frac{t^2}{2\sigma^2}}$ for any $t\geq 0$.  
\end{corollary}
